# Supplementary material for: Knowledge-Guided Wasserstein Distributionally Robust Optimization
Source: arXiv:2502.08146 source file (2025-02-12)
Supplement: Supplementary file 1 [file appendix.tex]

\section{Appendix}
